# Supplementary material for: Inducing $n$- and $p$-type thermoelectricity in oxide superlattices by strain tuning of orbital-selective transport resonances
Source: arXiv:1812.00503 ancillary file (2019-04-17)
Supplement: Supplementary file 1 [file Supplement.pdf]

# Inducing $n$- and $p$-type thermoelectricity in oxide superlattices by strain tuning of orbital-selective transport resonances
# – Supplemental Material –

Benjamin Geisler and Rossitza Pentcheva
*Department of Physics and Center for Nanointegration (CENIDE), Universität Duisburg-Essen, Lotharstr. 1, 47057 Duisburg, Germany*

## I. STRUCTURAL AND MAGNETIC INFORMATION

Figure 1 shows relative total energies of $(\mathrm{LNO})_3/(\mathrm{LAO})_1(001)$ SLs as functions of the substrate lattice parameter $a$, comparing $a^-a^-c^-$- and $a^-a^-c^+$-derived octahedral rotation patterns. For strong compressive strain, the octahedral rotations around the $a$ axes almost vanish if starting the ionic relaxation from a $a^-a^-c^-$ pattern; in the $a^-a^-c^+$ case, the initial pattern is basically preserved, but the $AlO_6$ octahedra flip to an antiferrodistortive rotation around the $c$ axis with respect to the $NiO_6$ octahedra. For $a \geq 3.85$ Å, an initial $a^-a^-c^+$ pattern relaxes to $a^-a^-c^0$, whereas an initial $a^-a^-c^-$ pattern leads to significant rotations around all three axes for $a \geq 3.70$ Å.

The vertical La-La distances shown in Fig. 2 reflect the decreasing trend of $c(a)$ (see Fig. 1 in the main text) with increasing substrate lattice constant $a$ (i.e., increasing epitaxial strain). The slope is higher for the Ni-related distances than for the Al-related one.

The volumes of the central $NiO_6$ octahedra become larger than those of the interfacial ones close to $a \approx 3.80$ Å (Fig. 2), i.e., close to the inflection point $a_\mathrm{i}$ of the $c(a)$ curve. This is accompanied by an increase of the central Ni spin magnetic moments and coincides with the appearance of octahedral rotations around the $a$ axes, as described in the main text.

The interfacial Ni spin magnetic moments, which are displayed in Fig. 2 as well, show almost no dependence on epitaxial strain, varying only between 1.05 and 1.08 $\mu_\mathrm{B}$, values slightly larger than the bulk LNO value of 1.04 $\mu_\mathrm{B}$. In contrast, the magnetic moment of the central Ni ions increases strongly from 0.80 to 1.17 $\mu_\mathrm{B}$ for the present range of substrate lattice constants. The local magnetic moments (Fig. 2) and the orbital polarization (Fig. 2 in the main text) show reversed strain dependence concerning central and interfacial nickelate layers: While the orbital polarization exhibits the strongest changes with strain at the interfaces, the local magnetic moments vary strongest in the central nickelate layers.

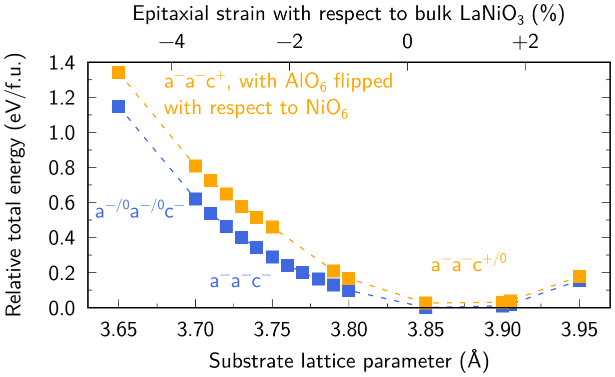


Figure 1. Relative total energies of $(\mathrm{LNO})_3/(\mathrm{LAO})_1(001)$ SLs for several substrate lattice parameters $a$, comparing $a^-a^-c^-$-derived (blue) and $a^-a^-c^+$-derived (orange) octahedral rotation patterns.

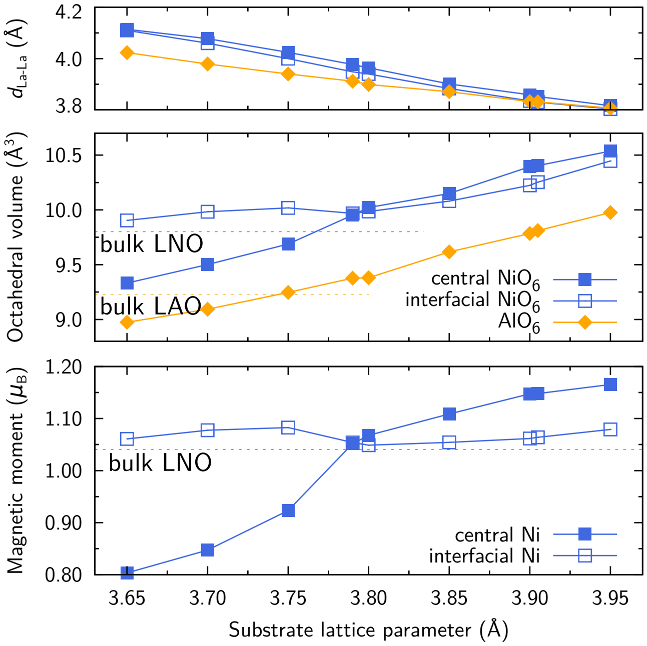


Figure 2. Vertical (i.e., in [001] direction) La-La distances, volumes of the $NiO_6$ and $AlO_6$ octahedra, and local Ni spin magnetic moments in different layers as functions of the substrate lattice parameter $a$ in $(\mathrm{LNO})_3/(\mathrm{LAO})_1(001)$ SLs.

## II. ELECTRONIC ASPECTS

The orbital polarization displayed in Fig. 2 in the main text is calculated from the orbital occupations $n$. Since in the Quantum Espresso code the orbital occupations are rendered by projecting onto orbitals that are aligned with the Cartesian coordinate system ($\tilde{n}$), some error is introduced for systems exhibiting octahedral tilts as in our case. In particular, the $t_{2g}$ orbitals, which should be fully occupied for $Ni^{3+}$, show an underestimation which is used to correct the occupation of the

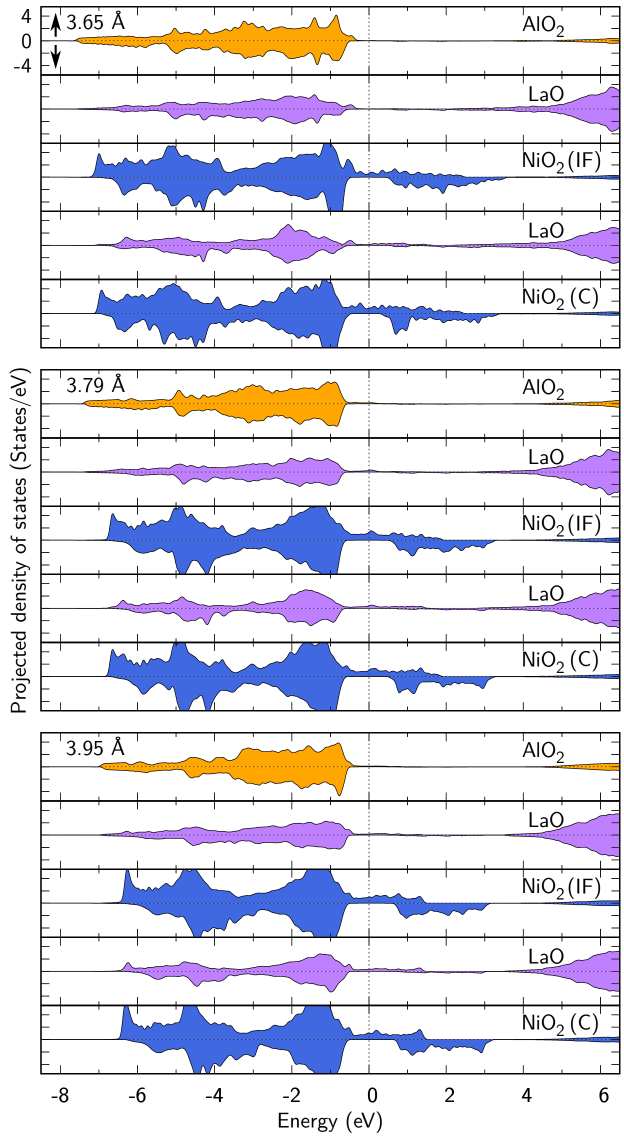


Figure 3. Layer- and spin-resolved densities of states of $(\mathrm{LNO})_3/(\mathrm{LAO})_1(001)$ SLs at $a = 3.65$ (top), 3.79 (middle), and 3.95 Å (bottom).

$e_g$ orbitals in a simple intuitive model:

$$n(3d_{x^2-y^2}) = \tilde{n}(3d_{x^2-y^2}) - (2 - \tilde{n}(3d_{xy})),$$
$$n(3d_{z^2}) = \tilde{n}(3d_{z^2}) - (4 - \tilde{n}(3d_{xz}) - \tilde{n}(3d_{yz})).$$

With this correction, we obtain a variation of the orbital polarization with the substrate lattice constant that is also consistent with experimental findings [1].

Figure 3 in the main text displays the integrated local density of states, which is is defined as [2–4]

$$\varrho(\vec{r}) = \int_{\varepsilon_1}^{\varepsilon_2} |\mathrm{d}\varepsilon| \sum_{n\vec{k}} |\psi_{n\vec{k}}(\vec{r})|^2 \, \delta(\varepsilon - \varepsilon_{n\vec{k}} + E_\mathrm{F}),$$

along a $(100)$ plane cutting through the Ni and Al sites. Here, $\psi_{n\vec{k}}$ and $\varepsilon_{n\vec{k}}$ are the Kohn-Sham states and energies of the system, respectively.

Figure 3 shows layer- and spin-resolved densities of states of $(\mathrm{LNO})_3/(\mathrm{LAO})_1(001)$ SLs for different substrate lattice parameters. Note the large band gap in the minority spin channel, which implies that only the majority bands are of relevance here. The valence band maximum of LAO is located $\sim 0.6$ eV below $E_\mathrm{F}$ (on average), see also Ref. 5

Figure 4 compares the majority spin band structure of $(\mathrm{LNO})_3/(\mathrm{LAO})_1(001)$ SLs for two different substrate lattice parameters to that of bulk LNO. While the Ni $3d_{x^2-y^2}$-derived states resemble bulk LNO, the Ni $3d_{z^2}$-derived states deviate significantly from bulk owing to the single LAO spacer layer. Instead, distinct quantum well states form.

Some of the substrates suggested in Fig. 4 in the main text are not (pseudo)cubic, but have an orthorhombic structure. We explored the impact of such an orthorhombic substrate on the electronic structure and total energy of $(\mathrm{LNO})_3/(\mathrm{LAO})_1(001)$ SLs exemplarily for $\mathrm{GdAlO_3}$ by setting the two in-plane lattice parameters to 5.247 Å and 5.304 Å (Ref. 6) and found only minor quantitative differences to the case of a $\sqrt{2} \cdot 3.73$ Å $\times \sqrt{2} \cdot 3.73$ Å cell (i.e., approximating the substrate to be pseudocubic).

## III. THERMOELECTRIC PROPERTIES

The thermoelectric properties are obtained in linear response by using the approach of Sivan and Imry [7]. The central quantity is the energy- and spin-resolved transmission (transport distribution) $\mathcal{T}_\sigma(E)$ which we determine by using the the BoltzTraP code [8].

From the *ab initio* electronic structure $\varepsilon_{i,\vec{k},\sigma}$ we calculate the group velocities in different directions $\vec{e}$, which then enter the corresponding energy- and spin-resolved transmission,

$$\mathcal{T}_\sigma(E) = \frac{e^2}{N} \sum_{i,\vec{k}} \delta(E - \varepsilon_{i,\vec{k},\sigma}) \left( \frac{1}{\hbar} \, \vec{e} \cdot \vec{\nabla}_k \, \varepsilon_{i,\vec{k},\sigma} \right)^2,$$

where $N$ is the total number of calculated $\vec{k}$ points. Within the common approximation of constant relaxation time $\tau$, the electrical conductivity can be expressed as

$$\sigma_\sigma(T,\mu) = -\frac{\tau}{\Omega} \int \mathrm{d}E \, \frac{\partial f}{\partial E} \, \mathcal{T}_\sigma(E),$$

where $\Omega = a^2 c$ is the volume of the considered supercell and $f = f_{\mu,T}(E)$ denotes the Fermi distribution function. The total conductivity is simply $\sigma = \sigma_\uparrow + \sigma_\downarrow$. The spin-projected Seebeck coefficients take on the form

$$S_\sigma(T,\mu) = -\frac{1}{eT} \frac{\int \mathrm{d}E \, \frac{\partial f}{\partial E} \, (E-\mu) \, \mathcal{T}_\sigma(E)}{\int \mathrm{d}E \, \frac{\partial f}{\partial E} \, \mathcal{T}_\sigma(E)}.$$

With these quantities the effective (charge) Seebeck coefficient can be expressed as

$$S = \frac{\sigma_\uparrow S_\uparrow + \sigma_\downarrow S_\downarrow}{\sigma_\uparrow + \sigma_\downarrow},$$

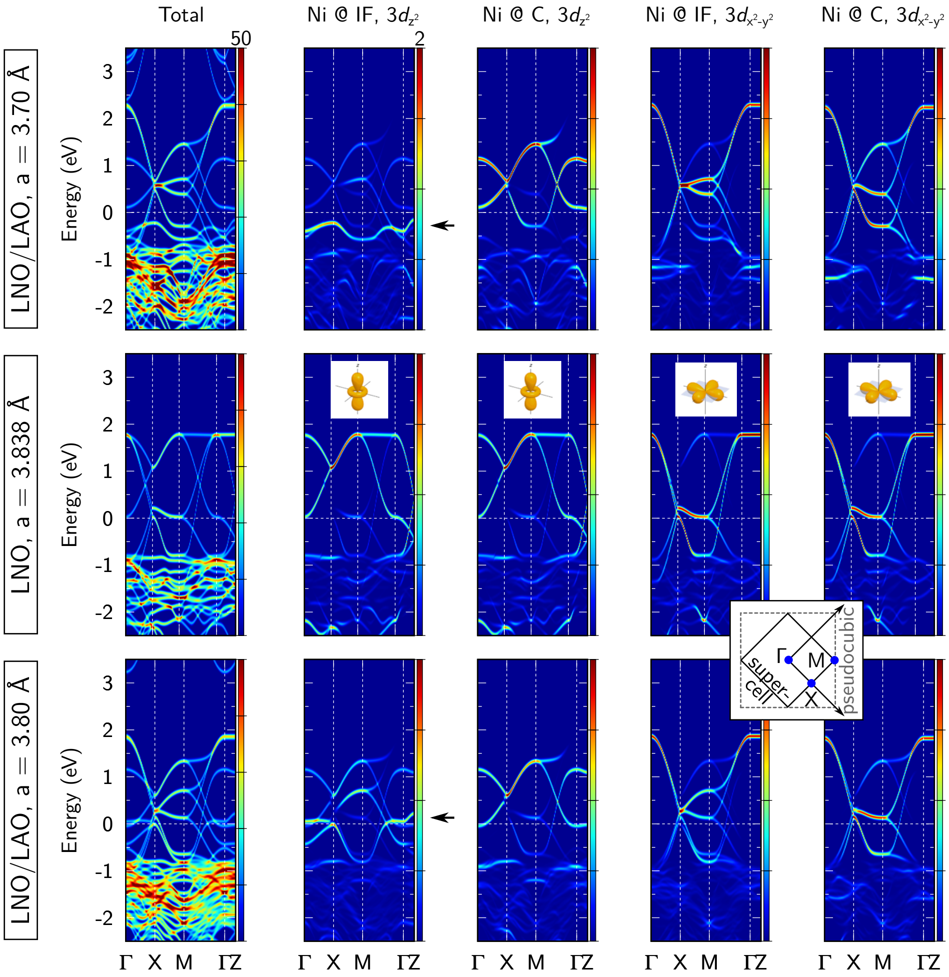


Figure 4. Majority spin band structures (total and projections on the two $e_g$ orbitals at interfacial and central Ni sites) of (LNO)$_3$/(LAO)$_1$(001) SLs (40 atoms) at $a = 3.70$ and 3.80 Å and of a bulk LNO supercell ($\sqrt{2}a \times \sqrt{2}a \times 2a$, 20 atoms) at the lattice parameter of the pseudocubic cell, $a = a_{\mathrm{LNO}} = 3.838$ Å. The inset clarifies the relation between the pseudocubic and our supercell Brillouin zone. While the Ni $3d_{x^2-y^2}$-derived states resemble bulk LNO, the Ni $3d_{z^2}$-derived states deviate significantly from bulk LNO due to the reduced symmetry and confinement induced by the single LAO spacer layer. The second Ni $3d_{z^2}$-derived quantum well state, which plays an important role here, is marked by black arrows. – The band structures correspond to $\vec{k}$-resolved densities of states, in which each electronic state is represented by a broadened delta distribution of weight one (total) or a weight equal to the projection of the respective wave function on $3d_{z^2}$ orbitals at different Ni sites (projected). The color scales are in units of $1/\mathrm{eV}$.

treating the two spin channels as parallel connected resistors. Note that the Seebeck coefficient does *not* depend on $\tau$ and is a measure for the asymmetry of the transmission around the chemical potential $\mu$.

Finally, the transmission allows also to calculate the electronic contribution to the thermal conductivity,

$$\kappa_{\mathrm{el}}(T,\mu) = -\frac{\tau}{e^2 T\Omega} \int \mathrm{d}E \, \frac{\partial f}{\partial E} \, (E-\mu)^2 \, \{\mathcal{T}_\uparrow(E) + \mathcal{T}_\downarrow(E)\} \, .$$

The position of the chemical potential $\mu(T)$ plays an important role for the thermoelectric properties of a given system [9]. Particularly if the system exhibits a band gap, $\mu(T)$ can vary by several hundred meV. However, owing to the two-dimensional metallic character of the present (LNO)$_3$/(LAO)$_1$(001) SLs, $\mu(T)$ varies by only $\sim 20$ meV in the temperature range considered here, and we set it to $E_{\mathrm{F}}$ for simplicity.

The thermoelectric figure of merit is defined as $ZT = \sigma S^2 T/\kappa_{\mathrm{total}}$, where $\kappa_{\mathrm{total}} = \kappa_{\mathrm{el}} + \kappa_{\mathrm{ph}}$ is the sum of electronic and phonon contribution to the thermal conductivity. The electronic figure of merit $ZT|_{\mathrm{el}}$, which we compare for different systems in Table 1 in the main text, is an upper limit of $ZT$ neglecting the phonon contribution to the thermal conductivity, $\kappa_{\mathrm{ph}} = 0$. As the Seebeck coefficient, $ZT|_{\mathrm{el}}$ does not depend on $\tau$. For the experimental LNO bulk values [10], using the measured $\kappa_{\mathrm{total}} \approx 0.11$ W/K cm at 300 K leads to $ZT = 0.009$. We additionally estimated $\kappa_{\mathrm{el}} \approx \kappa_{\mathrm{Wiedemann\text{-}Franz}} = 0.075$ W/K cm from the measured electrical conductivity at 300 K by using the Wiedemann-Franz law, resulting in $ZT|_{\mathrm{el}} = 0.013$. As expected for a metal, the largest part of the thermal conductivity stems from the electronic contribution $\kappa_{\mathrm{el}}$.

[1] M. Wu, E. Benckiser, M. W. Haverkort, A. Frano, Y. Lu, U. Nwankwo, S. Brück, P. Audehm, E. Goering, S. Macke, V. Hinkov, P. Wochner, G. Christiani, S. Heinze, G. Logvenov, H.-U. Habermeier, and B. Keimer, Strain and composition dependence of orbital polarization in nickel oxide superlattices, Phys. Rev. B **88**, 125124 (2013).

[2] B. Geisler and P. Kratzer, Atomic-scale detection of magnetic impurity interactions in bulk semiconductors, Phys. Rev. B **92**, 100407(R) (2015).

[3] B. Geisler and P. Kratzer, Strain stabilization and thickness dependence of magnetism in epitaxial transition metal monosilicide thin films on Si(111), Phys. Rev. B **88**, 115433 (2013).

[4] B. Geisler, P. Kratzer, T. Suzuki, T. Lutz, G. Costantini, and K. Kern, Growth mode and atomic structure of MnSi thin films on Si(111), Phys. Rev. B **86**, 115428 (2012).

[5] B. Geisler and R. Pentcheva, Confinement- and strain-induced enhancement of thermoelectric properties in $LaNiO_3/LaAlO_3(001)$ superlattices, Phys. Rev. Materials **2**, 055403 (2018).

[6] K.-H. Hellwege and A. M. Hellwege, eds., *Landolt-Börnstein, New Series*, Vol. III/4a (Springer-Verlag, Berlin, Heidelberg, New York, 1970).

[7] U. Sivan and Y. Imry, Multichannel Landauer formula for thermoelectric transport with application to thermopower near the mobility edge, Phys. Rev. B **33**, 551 (1986).

[8] G. K. H. Madsen and D. J. Singh, BoltzTraP. A code for calculating bandstructure dependent quantities, Comput. Phys. Commun. **175**, 67 (2006).

[9] B. Geisler and P. Kratzer, Spincaloric properties of epitaxial $Co_2MnSi/MgO/Co_2MnSi$ magnetic tunnel junctions, Phys. Rev. B **92**, 144418 (2015).

[10] J.-S. Zhou, L. G. Marshall, and J. B. Goodenough, Mass enhancement versus stoner enhancement in strongly correlated metallic perovskites: $LaNiO_3$ and $LaCuO_3$, Phys. Rev. B **89**, 245138 (2014).
